# Supplementary material for: Active Velocity Estimation using Light Curtains via Self-Supervised Multi-Armed Bandits
Source: arXiv:2302.12597 source file (2023-05-29)
Supplement: Supplementary file 1 [file instructions.tex]

\section{Instructions}
\label{app:instructions}

\noindent Our supplementary materials contain the following:

\begin{enumerate}
    \item Appendix: \texttt{appendix.pdf}
    \item Overview video
    \item Qualitative videos
    \item Source code: \texttt{code.zip}
\end{enumerate}

\noindent The easiest way to access our web-demo is to view the online version hosted on this anonymous website: \href{\website}{\underline{\texttt{\website}}}

\noindent However, it can also be run locally:
\begin{enumerate}
    \item \texttt{cd} into the folder containing supplementary materials.
    \item Run \texttt{python -m http.server}
    \item Open \texttt{http://localhost:8000/} in a web browser.
\end{enumerate}
